# Supplementary material for: Universality, scaling and collapse in supercritical fluids
Source: arXiv:1902.08360 source file (2019-02-22)
Supplement: Supplementary file 1 [file Supplementary_190221.pdf]

# Supplementary Materials for “Universality, Scaling and Collapse in Supercritical Fluids”

Min Young Ha, Tae Jun Yoon, Tsvi Tlusty, YongSeok Jho and Won Bo Lee

**Molecular Dynamics (MD) Simulations**

All MD simulations were performed using Large-scale Atomic/Molecular Massively Parallel Simulator (LAMMPS)[1]. Unless otherwise mentioned, 2,197 particles were used, interacting via pairwise Lennard-Jones (LJ) potential:

$$\phi(r_{ij}) = 4\epsilon\left[\left(\frac{\sigma}{r_{ij}}\right)^{12} - \left(\frac{\sigma}{r_{ij}}\right)^{6}\right], \tag{S1}$$

under periodic boundary condition for all three Cartesian directions. The potential was truncated at the cutoff distance of $r_{\mathrm{cut}} = 3.0\sigma$, and standard tail correction was applied assuming that the radial distribution function is unity beyond $r_{\mathrm{cut}}$. Lennard-Jones parameters $\varepsilon$ and $\sigma$ provide natural units of energy and length scales. Along with particle unit mass $m$, one can define the standard Lennard-Jones unit: $t^* = t\sqrt{\epsilon/m\sigma^2}$ for time, $T^* = k_B T/\epsilon$ for temperature, $P^* = \sigma^3 P/\epsilon$ for pressure, etc. Newtonian equation of motion was integrated via velocity-Verlet algorithm[2], with time step of 0.001. Nose-Hoover thermostat and barostat were used to maintain the temperature and pressure of the system at the desired value[3]. The initial positions of particles were randomly distributed and then relaxed using conjugate gradient methods to avoid divergence of potential energy. Velocities of particles were initialized according to Maxwell-Boltzmann distribution with zero-mean, to avoid momentum bias.

For every data point reported in this work, the system was equilibrated for 1,000,000 steps, and then production run was performed for 10,000,000 steps. Virial pressure in *NVT* ensemble and system volume in *NPT* ensemble was calculated every time step, and reported values of these properties are time averages during the production run. For the machine learning analysis, to minimize the correlation between snapshots, the positions of particles were dumped every 10,000 steps. Voronoi tessellation of snapshots were performed using VORO++ library[4].

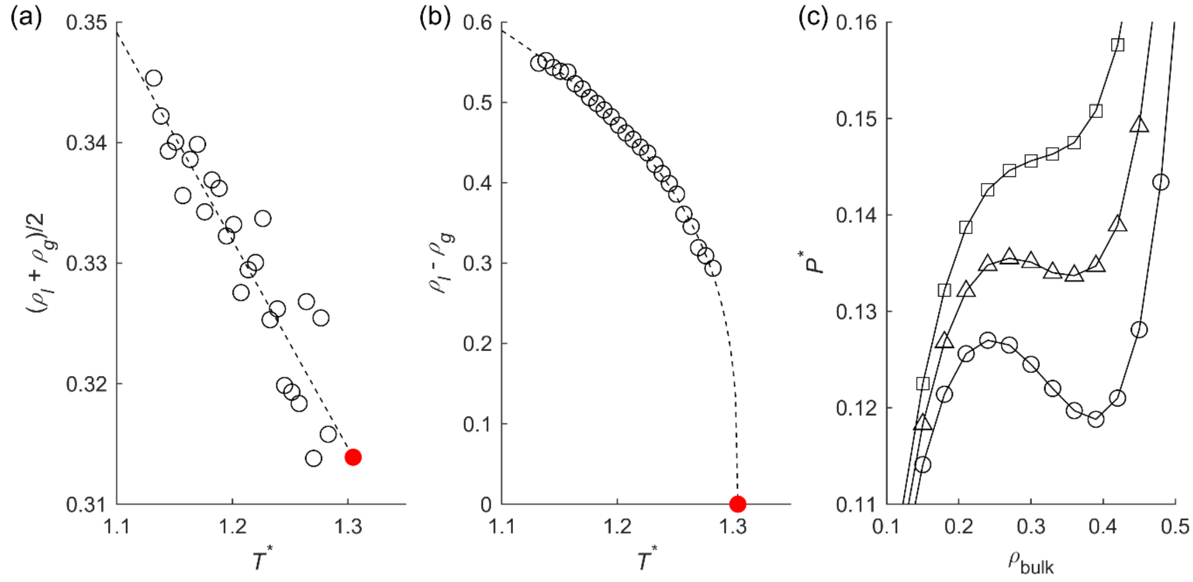


**Figure S1. Critical point estimation.** (a, b) The law of rectilinear diameters. Empty circles denote data acquired from simulation data, and the dashed lines denote numerical fitting to equations (2) and (3). Red circles denote the critical point, $(T_c^*, \rho_c^*) = (1.3047, 0.3139)$. (c) Van der Waals hypothesis. Circles, triangles and squares denote $T^* = 1.31$, $T^* = 1.33$ and $T^* = 1.35$, respectively. The estimated critical point is $(T_c^*, P_c^*, \rho_c^*) = (1.3449, 0.1428, 0.3110)$.

**Critical Point Estimation**

The critical temperature $(T_c)$, pressure $(P_c)$ and density $(\rho_c)$ are weakly dependent on the system size[5] and the treatment of interatomic potentials[6], hence it should be determined before performing near-critical simulations. To determine the critical parameters, we used two methods and compared their results: the law of rectilinear diameters[7], and van der Waals hypothesis[5].

The law of rectilinear diameter states that:

$$\frac{\rho_g + \rho_l}{2} = \rho_c + A(T_c - T), \tag{S2}$$

where $\rho_g$ and $\rho_l$ are saturated vapor and liquid densities, $\rho_c$ and $T_c$ are the critical density and temperature, and $A$ is the numerical fitting parameter. In addition, near-critical temperature and density follow the scaling law:

$$\rho_l - \rho_g = B(T_c - T)^{\beta}, \tag{S3}$$

where $\beta$ is the critical exponent and $B$ is acquired from numerical fitting. Densities of saturated vapor and liquid can be acquired from Gibbs ensemble Monte Carlo simulations, of which results are shown in Fig. S1(a) and (b). The critical temperature and density are $T_c^* = 1.3047$ and $\rho_c^* = 0.3139$. The critical pressure was obtained from the ensemble average of virial pressure in *NVT* ensemble with $T = T_c$ and $\rho = \rho_c$, which resulted in $P_c^* = 0.1202$.

Van der Waals hypothesis requires $\partial P/\partial\rho = \partial^2 P/\partial\rho^2 = 0$ at the critical point. Finite-sized, constant-volume MD simulation of isotropic systems does not spontaneously undergo liquid-gas phase separation, and unstable configurations with intermediate densities $(\rho_g < \rho < \rho_l)$ can be acquired. The simulations results are shown in Fig. S1(c), and interpolation results in critical parameters of $T_c^* = 1.3449$, $\rho_c^* = 0.3110$, and $P_c^* = 0.1428$. Note that while critical temperatures and densities of two different methods agree reasonably, critical pressures show relatively large discrepancy, due to strong temperature dependence of pressure in near-critical condition. These values can also be compared to the reported critical point of fluid interacting via full LJ potential[8]: $T_c^* = 1.326 \pm 0.002$, $\rho_c^* = 0.316 \pm 0.002$, and $P_c^* = 0.1279 \pm 0.0006$.

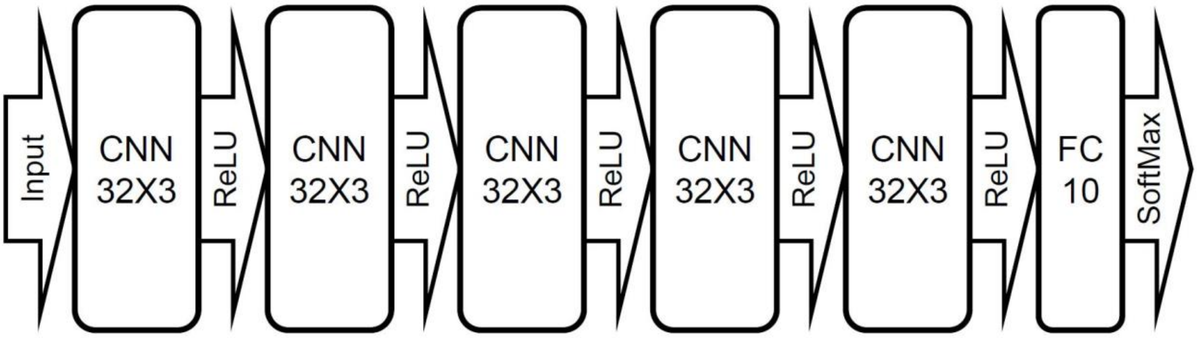


**Figure S2. Neural network architecture.** CNN block denotes the one-dimensional convolutional neural network layer, with 32 filters of kernel size 3. FC block denotes fully connected feed-forward neural network layer with 10 nodes. Arrow-shaped blocks denote rectified linear unit (ReLU) and softmax activation functions. All CNN layers were padded with zero entries at ends to maintain the data shape, and dropout was performed after the last CNN layer with probability of 0.25.

**Neural Network Architecture and Training**

In this work, as in our previous study[9], deep convolutional networks[10] motivated by VGGNet architecture[11] were used to classify liquid-like and gas-like particles coexisting in supercritical fluid. The architecture of the neural network is shown in Fig. S2. Instead of using a single neural network, we trained 24 neural networks with the same architecture, where the neural networks were trained with different permutations of training data.

The input into the neural network is a $2 \times 3$ matrix, $M_i$, which represents the local environment of $i^{\text{th}}$ particle. The first and second rows denote the statistics of $i^{\text{th}}$ particle and its nearest neighbor, respectively. The first column is the distance from the $i^{\text{th}}$ particle; the second column is the inverse volume of the Voronoi cell; the third column is the number of Voronoi neighbors, or equivalently, the number of faces of the Voronoi polyhedron.

The neural networks were trained with local structure matrices of 21,970,000 particles sampled from saturated liquid and vapor phases at $T/T_c = 0.97$, of which densities acquired from Gibbs-ensemble Monte Carlo simulation[7]. 20% of the data were reserved for cross-validation, and accuracies after training were $0.95 \pm 0.002$. The trained neural networks could classify saturated liquid and vapor particles generated at $T/T_c = 0.9$ with 100% accuracy.

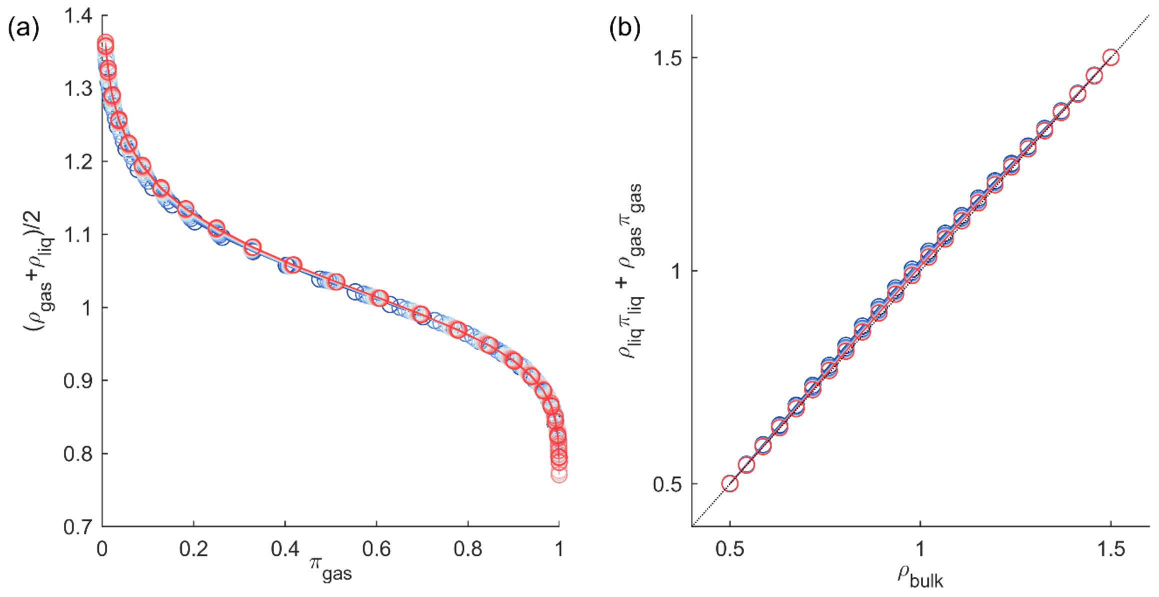


**Figure S3. Empirical relations between liquid-like and gas-like state densities.** (a) Average of gas-like and liquid-like densities are uniquely determined by $\pi_{\text{gas}}$, and is denoted $g_1(\pi)$: see equation S7. Different colors denote different temperatures, where the red colors mark higher temperatures than blue colors. (b) Weighted average of gas-like and liquid-like densities equals the bulk density, see equation S8. The black guiding line is the identity function, $\rho_{\text{liq}}\pi_{\text{liq}} + \rho_{\text{gas}}\pi_{\text{gas}} = \rho_{\text{bulk}}$.

## Densities of Gas-like and Liquid-like States

Since machine learning classifier labels individual particles as liquid-like or gas-like, it is possible to calculate the averaged properties of the two microstates. Let $v_i$ denote the Voronoi volume of the $i^{\text{th}}$ particle, and let $l_i$ express the label of the particle: $l_i$ is 0 and 1 for gas-like and liquid-like particles, respectively. We define the densities of gas-like and liquid-like states as follows:

$$\rho_{\text{gas}} = \frac{N_{\text{gas}}}{V_{\text{gas}}} = \frac{\sum_{i=1}^{N} \delta(l_i)}{\sum_{i=1}^{N} v_i \delta(l_i)}, \tag{S4}$$

$$\rho_{\text{liq}} = \frac{N_{\text{liq}}}{V_{\text{liq}}} = \frac{\sum_{i=1}^{N} \delta(l_i - 1)}{\sum_{i=1}^{N} v_i \delta(l_i - 1)}, \tag{S5}$$

where $\delta(x)$ is one for $x = 0$, and zero otherwise. Note that the sum of Voronoi volumes equals the system volume, i.e. $\sum_i v_i = V$. Along with the conservation of particle, $N_{\text{gas}} + N_{\text{liq}} = N$, this leads to:

$$\frac{1}{\rho_{\text{bulk}}} = \frac{V}{N} = \frac{V_{\text{liq}}}{N} + \frac{V_{\text{gas}}}{N} = \frac{V_{\text{liq}}}{N_{\text{liq}}}\frac{N_{\text{liq}}}{N} + \frac{V_{\text{gas}}}{N_{\text{gas}}}\frac{N_{\text{gas}}}{N} = \frac{\pi_{\text{liq}}}{\rho_{\text{liq}}} + \frac{\pi_{\text{gas}}}{\rho_{\text{gas}}}. \quad \text{(S6)}$$

Studying the microstate densities at different points on phase diagram, we found two interesting relations regarding $\rho_{\text{bulk}}$, $\rho_{\text{liq}}$ and $\rho_{\text{gas}}$. Fig. S3(a) shows that the arithmetic mean of the two densities are uniquely determined by the number fraction of microstates, $\pi_{\text{gas}}$, regardless of the specific position at the phase diagram. In the main text, we expressed this relationship by defining a generic function $g_1(\pi)$:

$$\frac{\rho_{\text{gas}} + \rho_{\text{liq}}}{2} = g_1(\pi). \quad \text{(S7)}$$

Moreover, Fig. S3(b) shows that instead of the conservation results of equation S6, a more simple and intuitive relation exists between the densities:

$$\rho_{\text{bulk}} = \rho_{\text{liq}}\pi_{\text{liq}} + \rho_{\text{gas}}\pi_{\text{gas}}. \quad \text{(S8)}$$

Equation S8 can be understood by studying the deviation of average densities from their values at SGLB, the loci of $\pi_{\text{gas}} = 0.5$. First, denote the average density of gas-like and liquid-like states at SGLB as $\rho_{\text{gas}}^{\text{o}}$ and $\rho_{\text{liq}}^{\text{o}}$. From Fig. S3(a) and equation S8, an approximate formula arises:

$$\frac{\rho_{\text{gas}}^{\text{o}} + \rho_{\text{liq}}^{\text{o}}}{2} \cong \rho_c. \quad \text{(S9)}$$

Alternatively, one can write this as $\rho_{\text{gas}}^{\text{o}} \cong \rho_c - \Delta\rho^{\text{o}}$ and $\rho_{\text{liq}}^{\text{o}} \cong \rho_c + \Delta\rho^{\text{o}}$. Moving away from SGLB, the deviation from SGLB can be expressed as:

$$\rho_{\text{gas}} = \rho_{\text{gas}}^{\text{o}} + \Delta\rho_{\text{gas}} = \rho_c - \Delta\rho^{\text{o}} + \Delta\rho_{\text{gas}}, \quad \text{(S10)}$$

$$\rho_{\text{liq}} = \rho_{\text{liq}}^{\text{o}} + \Delta\rho_{\text{liq}} = \rho_c + \Delta\rho^{\text{o}} + \Delta\rho_{\text{liq}}. \quad \text{(S11)}$$

Equating equations S6 and S8 is equivalent to showing that

$$\rho_{\text{gas}}\rho_{\text{liq}} = \left(\pi_{\text{gas}}\rho_{\text{gas}} + \pi_{\text{liq}}\rho_{\text{liq}}\right)\left(\pi_{\text{gas}}\rho_{\text{liq}} + \pi_{\text{liq}}\rho_{\text{gas}}\right). \quad \text{(S12)}$$

Using equations S10 and S11, the LHS of equation S12 is

$$\begin{aligned}\rho_{\mathrm{gas}}\rho_{\mathrm{liq}} &= \rho_c^2 + \rho_c\left(\Delta\rho_{\mathrm{gas}} + \Delta\rho_{\mathrm{liq}}\right) + \Delta\rho^{\mathrm{o}}\left(\Delta\rho_{\mathrm{gas}} - \Delta\rho_{\mathrm{liq}}\right) - (\Delta\rho^{\mathrm{o}})^2 + \Delta\rho_{\mathrm{gas}}\Delta\rho_{\mathrm{liq}} \\ &= \rho_c^2 + \rho_c\left(\Delta\rho_{\mathrm{gas}} + \Delta\rho_{\mathrm{liq}}\right) + O(\Delta x^2), \qquad \text{(S13)}\end{aligned}$$

where the second-ordered deviation terms are assumed to be small compared to critical density, $\rho_c$, and packed into the $O(\Delta x^2)$ term. Expanding the RHS of equation S12,

$$\begin{aligned}&\left(\rho_{\mathrm{gas}}\pi_{\mathrm{gas}} + \rho_{\mathrm{liq}}\pi_{\mathrm{liq}}\right)\left(\rho_{\mathrm{gas}}\pi_{\mathrm{liq}} + \rho_{\mathrm{liq}}\pi_{\mathrm{gas}}\right) \\ &= \left(\frac{\rho_{\mathrm{gas}} + \rho_{\mathrm{liq}}}{2} + \Delta\pi\left(\rho_{\mathrm{liq}} - \rho_{\mathrm{gas}}\right)\right)\left(\frac{\rho_{\mathrm{gas}} + \rho_{\mathrm{liq}}}{2} - \Delta\pi\left(\rho_{\mathrm{liq}} - \rho_{\mathrm{gas}}\right)\right) \\ &= \left[\rho_c + \frac{\Delta\rho_{\mathrm{gas}} + \Delta\rho_{\mathrm{liq}}}{2} + \Delta\pi\left(2\Delta\rho^{\mathrm{o}} + \Delta\rho_{\mathrm{liq}} - \Delta\rho_{\mathrm{gas}}\right)\right] \\ &\qquad \times \left[\rho_c + \frac{\Delta\rho_{\mathrm{gas}} + \Delta\rho_{\mathrm{liq}}}{2} - \Delta\pi\left(2\Delta\rho^{\mathrm{o}} + \Delta\rho_{\mathrm{liq}} - \Delta\rho_{\mathrm{gas}}\right)\right] \\ &= \rho_c^2 + \rho_c\left(\Delta\rho_{\mathrm{gas}} + \Delta\rho_{\mathrm{liq}}\right) + O(\Delta x^2). \qquad \text{(S14)}\end{aligned}$$

Equations S13 and S14 show that equation S12 holds to the second order of deviation from SGLB ($\Delta\pi$, $\Delta\rho_{\mathrm{liq}}$, $\Delta\rho_{\mathrm{gas}}$). Hence, equation S8 can be justified to the second order of errors.

Expanding equation S8 with respect to SGLB,

$$\begin{aligned}\rho_{\mathrm{bulk}} &= \rho_{\mathrm{gas}}\pi_{\mathrm{gas}} + \rho_{\mathrm{liq}}\pi_{\mathrm{liq}} = \rho_{\mathrm{gas}}(0.5 - \Delta\pi) + \rho_{\mathrm{liq}}(0.5 + \Delta\pi) \\ &= \frac{\rho_{\mathrm{gas}} + \rho_{\mathrm{liq}}}{2} + \Delta\pi\left(\rho_{\mathrm{liq}} - \rho_{\mathrm{gas}}\right) \\ &= g_1(\pi) + \Delta\pi\left(\rho_{\mathrm{liq}}^{\mathrm{o}} - \rho_{\mathrm{gas}}^{\mathrm{o}}\right) + \Delta\pi\left(\Delta\rho_{\mathrm{liq}} - \Delta\rho_{\mathrm{gas}}\right). \qquad \text{(S15)}\end{aligned}$$

Note that $g_1(\pi)$ is defined in equation S7. The two additional terms in equation S15 are shown in Fig. S4. It can be found in Fig. S4(a) that $\Delta\rho_{\mathrm{liq}} - \Delta\rho_{\mathrm{gas}}$ is another function of number fraction, hence we express this term as $g_2(\pi)$:

$$\Delta\rho_{\mathrm{liq}} - \Delta\rho_{\mathrm{gas}} = g_2(\pi). \qquad \text{(S16)}$$

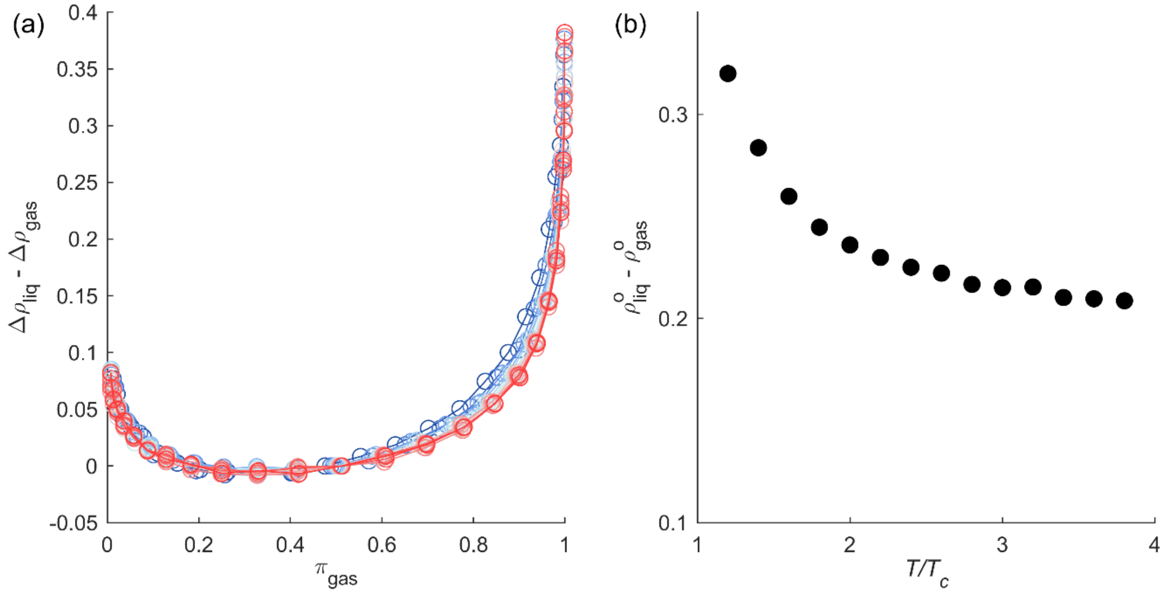


**Figure S4. Differences between liquid-like and gas-like densities.**

Moreover, Fig. S4(b) shows that $\rho^{\mathrm{o}}_{\mathrm{liq}} - \rho^{\mathrm{o}}_{\mathrm{gas}}$ is only weakly dependent on temperature, of which value slowly converges to a finite value in the $T \to \infty$ limit. Note that even in the close vicinity of the critical temperature, it does not increase more than numerical factor of two from the value at $T \to \infty$ limit. Hence, if the temperature range is not very wide, or far away from the critical value, $\rho^{\mathrm{o}}_{\mathrm{liq}} - \rho^{\mathrm{o}}_{\mathrm{gas}}$ can be roughly considered constant. As far as these conditions are met, one can claim that $\rho_{\mathrm{bulk}}$ is a function of $\pi_{\mathrm{gas}}$, and since the scaling relationships of $\pi_{\mathrm{gas}}$ were found in the main text, it is reasonable to expect that the same rescaling is possible for the density curves along isothermal or isobaric changes from the critical isochore.

Figures S5 and S6 show the density data of argon, carbon dioxide and water, acquired from NIST chemistry webbook database. They demonstrate that using the same scaling relationships of $\pi_{\mathrm{gas}}$, the density phase diagram of supercritical fluids can be rescaled into a single curve, provided that the temperature range is reasonable.

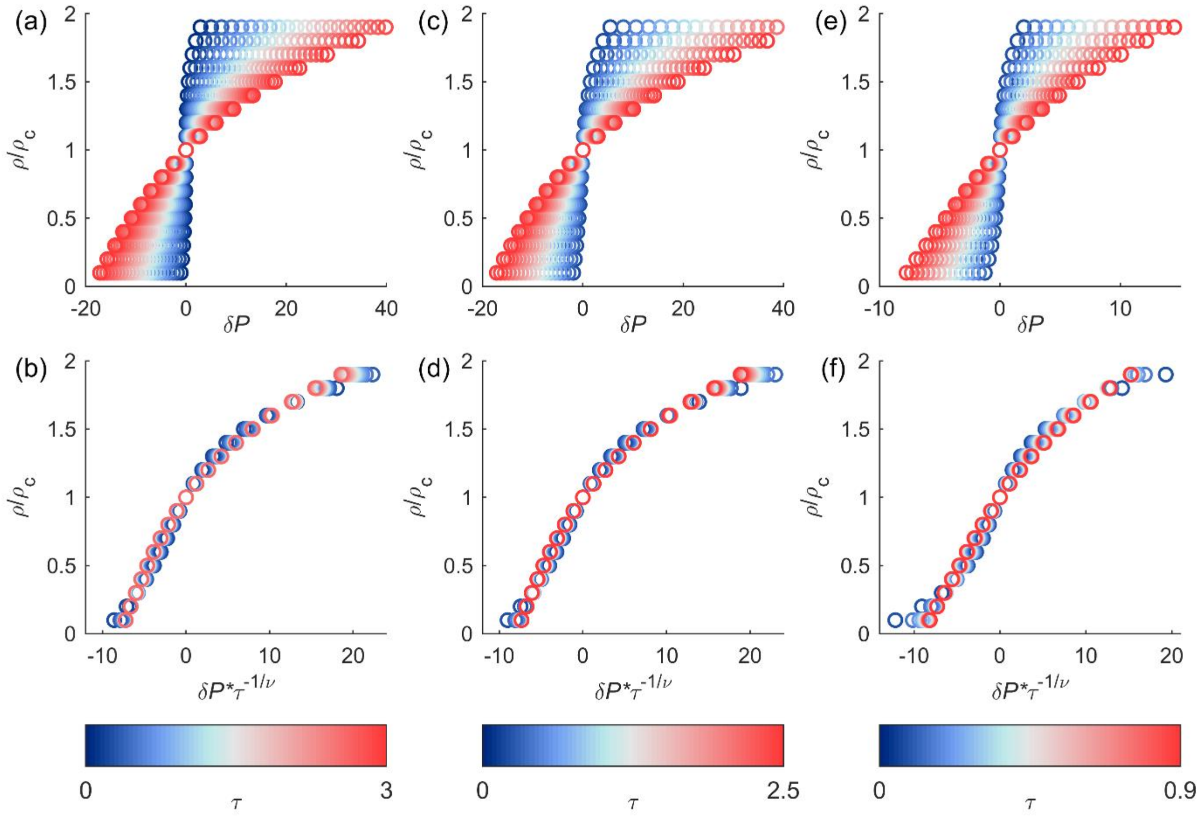


**Figure S5. Isothermal scaling of NIST density data.** (a) Raw density data of Ar. (b) Rescaled density data of Ar. (c) Raw density data of $CO_2$. (d) Rescaled density data of $CO_2$. (e) Raw density data of $H_2O$. (f) Rescaled density data of $H_2O$.

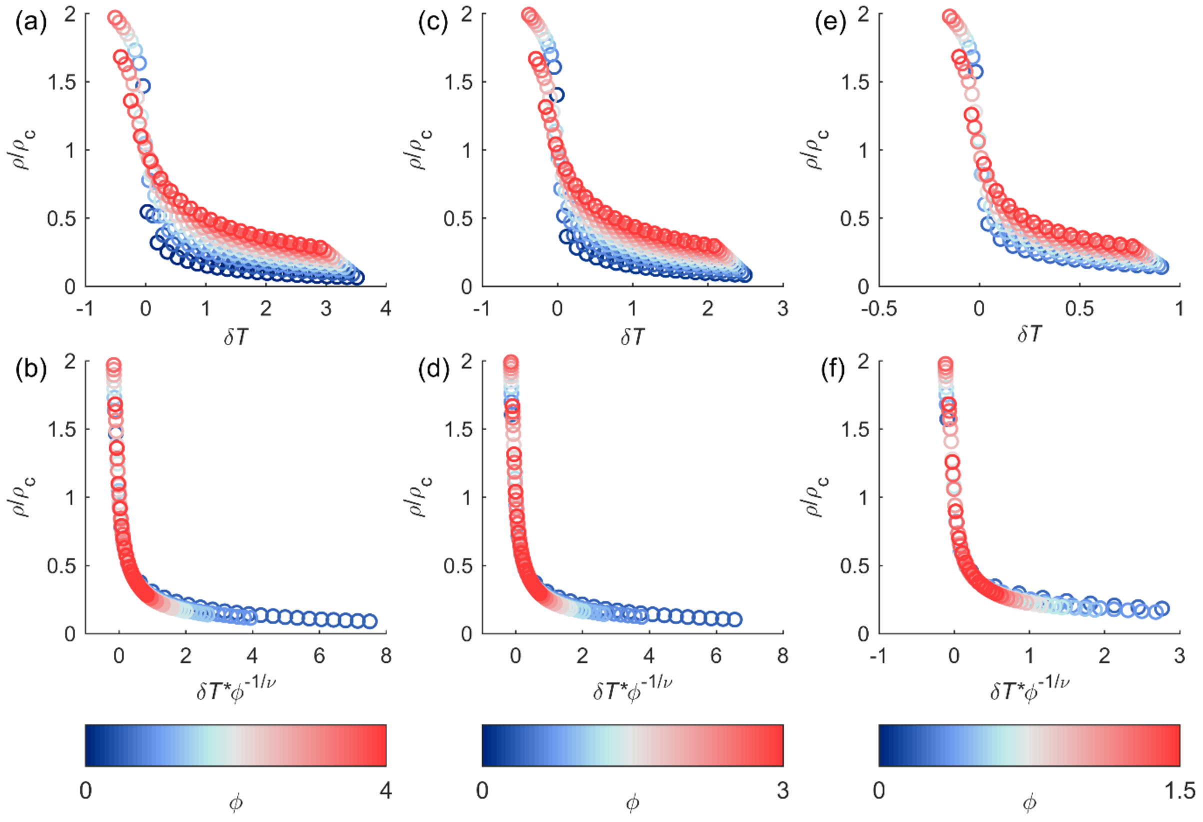


**Figure S6. Isobaric scaling of NIST density data.** (a) Raw density data of Ar. (b) Rescaled density data of Ar. (c) Raw density data of $CO_2$. (d) Rescaled density data of $CO_2$. (e) Raw density data of $H_2O$. (f) Rescaled density data of $H_2O$.

## References


1. Plimpton, S. Fast parallel algorithms for short-range molecular dynamics. *J. Comput. Phys.* **117,** 1–19 (1995).

2. Tuckerman, M. E., Alejandre, J., López-Rendón, R., Jochim, A. L. & Martyna, G. J. A Liouville-operator derived measure-preserving integrator for molecular dynamics simulations in the isothermal--isobaric ensemble. *J. Phys. A. Math. Gen.* **39,** 5629 (2006).

3. Shinoda, W., Shiga, M. & Mikami, M. Rapid estimation of elastic constants by molecular dynamics simulation under constant stress. *Phys. Rev. B* **69,** 134103 (2004).

4. Rycroft, C. Voro++: A three-dimensional Voronoi cell library in C++. (2009).

5. Heyes, D. M. & Woodcock, L. V. Critical and supercritical properties of Lennard--Jones fluids. *Fluid Phase Equilib.* **356,** 301–308 (2013).

6. Smit, B. Phase diagrams of Lennard-Jones fluids. *J. Chem. Phys.* **96,** 8639–8640 (1992).

7. Frenkel, D. & Smit, B. *Understanding molecular simulation: from algorithms to applications*. **1,** (Elsevier, 2001).

8. Potoff, J. J. & Panagiotopoulos, A. Z. Critical point and phase behavior of the pure fluid and a Lennard-Jones mixture. *J. Chem. Phys.* **109,** 10914–10920 (1998).

9. Ha, M. Y., Yoon, T. J., Tlusty, T., Jho, Y. & Lee, W. B. Widom Delta of Supercritical Gas--Liquid Coexistence. *J. Phys. Chem. Lett.* **9,** 1734–1738 (2018).

10. Goodfellow, I., Bengio, Y., Courville, A. & Bengio, Y. *Deep learning*. **1,** (MIT press Cambridge, 2016).

11. Simonyan, K. & Zisserman, A. Very deep convolutional networks for large-scale image recognition. *arXiv Prepr. arXiv1409.1556* (2014).
